# Supplementary material for: Computing Optimal Repairs for Functional Dependencies
Source: arXiv:1712.07705 source file (2017-12-20)
Supplement: Supplementary file 1 [file appendix-value-repair.tex]

\section{Details from Section 5}\label{app:proofs-value-repair}

\subsection{Proof of }

\section{Updates $A->B,B->A,B->C$}

In this section we prove the following lemma.

\begin{lemma}\label{lemma:updates-ab-ba-bc}
  Let $(\signature, \depset)$ be an FD schema, such that $\signature$ consists of a single relation $R(A,B,C)$ and $\depset=\set{A\rightarrow B, B\rightarrow A, B\rightarrow C}$. Then, the problem $\maxvrepfd{\signature}{\depset}$ is NP-hard.
\end{lemma}

The idea of our proof of Lemma~\ref{lemma:updates-ab-ba-bc} is similar to the idea of the proof of NP-hardness for the set of FDs $\depset=\set{A\rightarrow B, B\rightarrow C}$ in~\cite{DBLP:conf/icdt/KolahiL09}. We construct a reduction from the minimum vertex cover problem and prove that the size of the minimum vertex cover is $k$ if and only if the cost of the minimum v-repair for the constructed instance is $2|E|+k$ (where $E$ is the set of edges in the original graph). However, in this case, we have to prove some nontrivial results before we can use a similar proof to theirs for the reduction.

The input to minimum vertex cover problem is a graph $g$. The goal is to find a vertex cover $C$ for $g$ (a set of vertices that touches every edge in $g$), such that no other vertex cover $C'$ of $g$ contains less vertices than $C$ (that is, $|C'|<|C|$). This problem is known to be NP-hard.
 Given such an input, 
 we will construct the input 
 $I$ for our problem as follows.
 Let $V=\set{v_1,\dots,v_n}$ be the set of vertices in $g$ and let $E=\set{e_1,\dots,e_m}$ be the set of edges in $g$. For each edge $e_r=(v_i,v_j)$ in $E$, the instance $I$ will contain the following facts:
 \begin{itemize}
 \item
 $R(v_i,v_j,\val{0})$,
 \item
$R(v_j,v_i,\val{0})$.
 \end{itemize}
 In addition, for each vertex $v_i\in V$, the instance $I$ will contain the following fact:
  \begin{itemize}
 \item
 $R(v_i,v_i,\val{1})$,
 \end{itemize}
 
Let $C_{min}$ be a minimum vertex cover of $g$. We will now prove the following results:
 \begin{enumerate}
     %\item The cost of each v-repair of $I$ is at least $2|E|$.
     \item For each vertex cover $C$ of $g$ of size $k$, there is a v-repair of $I$ with a cost $2|E|+k$.
     \item No v-repair of $I$ has a cost $2|E|+k$ for some $k<|C_{min}|$.
 \end{enumerate}
  Then, we can conclude that the size of the minimum vertex cover of $g$ is $m$ if and only if the cost of the minimum v-repair of $I$ is $2|E|+m$.
 
% \begin{lemma}\label{lemma:updates-ab-ba-bc-min2E}
% The cost of each v-repair of $I$ is at least $2|E|$.
% \end{lemma}
% \begin{proof}
% Let $J$ be a v-repair of $I$, and let $\set{f_1,\dots f_l}$ be the set of facts of the form $R(v_i,v_j,\val{0})$ in $I$ that are not updated by $J$. Clearly, if this set is empty, then the cost of $J$ is at least $2|E|$, since there are exactly $2|E|$ facts of this form. If this set is not empty, then $J$ updates $2|E|-l$ facts of this form, and does not update $l$ facts of this form, for some $l\in\set{1,\dots,2|E|-1}$. Let $f_r$ be the fact $R(v_i,v_j,\val{0})$ for some $v_i,v_j\in V$. Note that there is a conflict between this fact and the fact $R(v_i,v_i,\val{1})$ (since they agree on the value of attribute $A$, but do not agree on the value of attribute $B$, thus they violate the FD $A\rightarrow B$). Therefore, if the fact $R(v_i,v_j,\val{0})$ is not updated, the fact $R(v_i,v_i,\val{1})$ must be updated. Hence, we update $2|E|-l$ facts of the form $R(v_i,v_j,\val{0})$ and at least $l$ facts of the form $R(v_i,v_i,\val{1})$, and the cost of $J$ is at least $2|E|-l+l=2|E|$.
% \end{proof}

\subsection{Proof of (1)}
We will now prove that for each vertex cover $C$ of $g$ of size $k$, there is a v-repair of $I$ with cost $2|E|+k$. Assume that $C$ is a vertex cover of $g$ that contain $k$ vertices. We can build a v-repair $J$ of $I$ as follows: for each edge $e_r=(v_i,v_j)$, if $v_i\in C$, then we will change the facts $R(v_i,v_j,\val{0})$ and $R(v_j,v_i,\val{0})$ to $R(v_i,v_i,\val{0})$. Otherwise, we will change these two facts to $R(v_j,v_j,\val{0})$ (note that in this case, since $v_i$ does not belong to the vertex cover, $v_j$ does). Moreover, for each vertex $v_i$ that belongs to $C$, we will change the fact $R(v_i,v_i,\val{1})$ to $R(v_i,v_i,\val{0})$. Note that if a vertex $v_i$ does not belong to $C$, the instance $J$ will not contain any fact of the form $R(v_i,v_i,\val{0})$, thus the fact $R(v_i,v_i,\val{1})$ does not agree on the value of $A$ or $B$ with any other fact in $J$, and is not in conflict with any other fact. On the other hand, if a node $v_i$ does belong to $C$, the instance $J$ will only contain facts of the form $R(v_i,v_i,\val{0})$ for $v_i$, since in this case we change the fact $R(v_i,v_i,\val{1})$ to $R(v_i,v_i,\val{0})$. Thus, $J$ is indeed a v-repair. Finally, for each edge $(v_i,v_j)\in E$ we update one cell in each of the facts  $R(v_i,v_j,\val{0})$ and $R(v_j,v_i,\val{0})$ ($2|E|$ cell updates), and for each vertex $V_i\in C$ we update one cell in the fact $R(v_i,v_i,\val{1})$ ($k$ cell updates), thus the cost of $J$ is $2|E|+k$.

\subsection{Proof of (2)}
\newcounter{counter}

In order to prove this part of the lemma (that is, that no v-repair of $I$ is of cost $2|E|+k$ for some $k<|C_{min}|$), we first have to prove the following lemma, which is a nontrivial part of the proof.

\begin{lemma}\label{lemma:comp-proof}
Let $J$ be a v-repair of $I$ that updates $t$ facts of the form $R(v_i,v_j,\val{0})$ for some $t<2|E|$. Then, there is a v-repair $J'$ of $I$, that updates at least $t+1$ facts of the form $R(v_i,v_j,\val{0})$, such that the cost of $J'$ is lower or equal to the cost of $J$.
\end{lemma}
\begin{proof}
Since it holds that $t<2|E|$, there is at least one fact $R(v_1,v_2,\val{0})$, for some $v_1,v_2\in V$ that is not updated by $J$. We will now show that we can build another v-repair $J'$, that updates the fact $R(v_1,v_2,\val{0})$ (as well as every fact that is updated by $J$), such that the cost of $J'$ is lower or equal to the cost of $J$. That is, $J'$ will update at least $t+1$ facts of the form $R(v_i,v_j,\val{0})$.

The fact $f_1=R(v_1,v_2,\val{0})$ is in conflict with the facts $f_2=R(v_1,v_1,\val{1})$ and $f_3=R(v_2,v_2,\val{1})$. Moreover, these two facts are in conflict with the fact $f_4=R(v_2,v_1,\val{0})$. We will now show that since the fact $f_1$ is not updated by $J$ and $J$ is consistent, $J$ must make at least four changes to the facts in $\set{f_2,f_3,f_4}$. The following holds: 
\begin{enumerate}
    \item To resolve the conflict between $f_1$ and $f_2$ (that agree only on the value of attribute $A$), we have to either change the value of attribute $A$ in $f_2$ to another value, or change the values of both attributes $B$ and $C$ to $v_2$ and $\val{0}$, respectively. In the first case, since $f_2$ is still in conflict with $f_4$ (as they only agree on the value of attribute $B$), we also have to change the value of attribute $B$ in one of $f_2$ or $f_4$. In the second case, $f_2$ and $f_4$ are no longer in conflict, thus we do not have to make any more changes. In both cases, the cost of the update is $2$.
    \item To resolve the conflict between $f_1$ and $f_3$ (that agree only on the value of attribute $B$), we have to either change the value of attribute $B$ in $f_3$ to another value, or change the values of both attributes $A$ and $C$ to $v_1$ and $\val{0}$, respectively. In the first case, since $f_3$ is still in conflict with $f_4$ (as they only agree on the value of attribute $A$), we also have to change the value of attribute $A$ in one of $f_3$ or $f_4$. In the second case, $f_3$ and $f_4$ are no longer in conflict, thus we do not have to make any more changes. In both cases, the cost of the update is $2$.
\end{enumerate} 
Note that the updates presented in $(1)$ and $(2)$ above are independent (as they change different attributes in different facts), thus we have to combine them to resolve all of the conflicts among the facts in $\set{f_1,f_2,f_3,f_4}$, and the total cost of updating the facts $f_2$, $f_3$ and $f_4$ in $J$ is at least $4$. Moreover, note that it is not necessary to change the value of attribute $A$ in both $f_3$ and $f_4$ or change the value of attribute $B$ in both $f_2$ and $f_4$, since changing just one of them resolves the conflict between the facts. If $J$ updates both of these values, then the cost of updating the facts $f_2$, $f_3$ and $f_4$ is increased by one for each pair of facts ($f_2$ and $f_4$, or $f_3$ and $f_4$) updated together. We will use this observation later in the proof.

Now, we will build an instance $J'$ that updates each one of the facts updated by $J$, as well as the fact $f_1$. We will prove that the cost of $J'$ is not higher than the cost of $J$. We will start by adding these four facts to $J'$:
\begin{enumerate}
    \item Instead of the fact $f_1$ ($R(v_1,v_2,\val{0})$), we will insert the fact $R(v_1,v_1,\val{0})$.
    \item Instead of the fact $f_2$ ($R(v_1,v_1,\val{1})$), we will insert the fact $R(v_1,v_1,\val{0})$.
    \item Instead of the fact $f_3$ ($R(v_2,v_2,\val{1})$), we will insert the fact $R(v_2,v_2,\val{0})$.
    \item Instead of the fact $f_4$ ($R(v_2,v_1,\val{0})$), we will insert the fact $R(v_2,v_2,\val{0})$.
    \setcounter{counter}{\value{enumi}}
\end{enumerate}
So far we only updated one cell in each of the four facts discussed above. Thus, the current cost is $4$. As mentioned above, the cost of changing these facts in $J$ is at least $4$, thus so far we did not exceed the cost of $J$. From now on, we will look at the rest of the facts in $J$ and insert each one of them to $J'$ (in some cases, only after updating them to resolve some conflict). 
\begin{enumerate}
    \setcounter{enumi}{\value{counter}}
    \item For each fact $f$ that appears in $J$ that is not in conflict with one of $R(v_1,v_1,\val{0})$ or $R(v_2,v_2,\val{0})$, we insert $f$ to $J'$.
    \setcounter{counter}{\value{enumi}}
\end{enumerate}
Clearly, $J'$ is consistent at this point, and since those facts are updated by $J'$ in exactly the same way they were updated by $J$, we did not exceed the cost of $J$. Each one of the remaining facts is in conflict with one of $R(v_1,v_1,\val{0})$ or $R(v_2,v_2,\val{0})$, thus we have to update it before inserting it to $J'$.
\begin{enumerate}
    \setcounter{enumi}{\value{counter}}
    \item Each fact $f$ such that $f[A]=v_1$ is in conflict with the fact $R(v_1,v_1,\val{0})$. Since the fact $R(v_1,v_2,\val{0})$ belongs to $J$ and $J$ is consistent, it holds that $f=R(v_1,v_2,\val{0})$. 
    There are a few possible cases:
        \begin{itemize}
            \item If the original fact $f$ (the fact in the instance $I$) was of the form $R(v_i,v_j,\val{0})$ for some $v_i\neq v_1$ and $v_j\neq v_2$, then $J$ updated two cells in this fact. We will replace this fact in $J'$ with the fact $R(v_1,v_1,\val{0})$. Note that the cost is the same (since we again update two cells).
            \item If the original fact $f$ was of the form $R(v_1,v_j,\val{0})$ for some $v_j\neq v_2$, then $J$ updated one cell in this fact. We will replace this fact in $J'$ with the fact $R(v_1,v_1,\val{0})$. Again, the cost is the same.
            \item If the original fact was of the form $R(v_i,v_2,\val{0})$ for some $v_i\neq v_1$, we will replace it with the fact $R(v_2,v_2,\val{0})$ with no additional cost.
            \item If the original fact was of the form $R(v_i,v_i,\val{1})$ for some $v_i\not\in\set{v_1,v_2}$ (we already handled the case where $v_i$ is one of $v_1$ or $v_2$), then $J$ updated three cells in this fact (the values in all of the attributes are different from the values in the fact $R(v_1,v_2,\val{0})$), and we will replace it with the fact $R(v_2,v_2,\val{0})$ with no additional cost.
        \end{itemize}
    \item Each fact $f$ such that $f[B]=v_2$ is in conflict with the fact $R(v_2,v_2,\val{0})$. Again, since the fact $R(v_1,v_2,\val{0})$ belongs to $J$ and $J$ is consistent, it holds that $f=R(v_1,v_2,\val{0})$. This case is symmetric to the previous one, thus we will not elaborate on all of the possible cases.
    \setcounter{counter}{\value{enumi}}
\end{enumerate}
So far, we inserted to $J'$ one fact (either $R(v_1,v_1,\val{0})$ or $R(v_2,v_2,\val{0})$) for each of the four facts in $\set{f_1,f_2,f_3,f_4}$, one fact for each fact in $J$ that is not in conflict with neither $R(v_1,v_1,\val{0})$ nor $R(v_2,v_2,\val{0})$, and one fact (again either $R(v_1,v_1,\val{0})$ or $R(v_2,v_2,\val{0})$) for each fact in $J$ that agrees with $R(v_1,v_1,\val{0})$ only on the value of attribute $A$ or agrees with $R(v_2,v_2,\val{0})$ only on the value of attribute $B$. It is left to insert each fact that agrees with $R(v_1,v_1,\val{0})$ on the value of attribute $B$ or agrees with $R(v_2,v_2,\val{0})$) on the value of attribute $A$.
\begin{enumerate}
    \setcounter{enumi}{\value{counter}}
    \item Each fact $f$ such that $f[A]=v_2$ is in conflict with the fact $R(v_2,v_2,\val{0})$. Note that in this case it holds that $f[B]\neq v_2$, since $J$ is consistent and also contains the fact $R(v_1,v_2,\val{0})$. Assume that $f$ is the fact $R(v_2,v_i,x)$ for some $v_i\in V$. Again, there are a few possible cases:
        \begin{itemize}
            \item  If the original fact $f$ (the fact in the instance $I$) was of the form $R(v_j,v_i',y)$ for some $v_j\neq v_2$ and $v_i'\neq v_i$, then $J$ updated at least two cells in this fact in $J$. We will replace this fact in $J'$ with the fact $R(v_2,v_2,\val{0})$, with no additional cost.
            \item If the original fact $f$ was of the form $R(v_2,v_i',\val{0})$ for some $v_i'\neq v_i$, then $J$ updated at least one cell in this fact (the value of attribute $B$). We will replace this fact in $J'$ with the fact $R(v_2,v_2,\val{0})$, with no additional cost.
            \item If the original fact $f$ was of the form $R(v_j,v_i,x)$ for some $v_j\neq v_2$, then $J$ updated at least one cell in this fact (the value of attribute $A$). We will replace this fact in $J'$ with the fact $R(y_i,v_i,\val{0})$, for some new value $y_i$ that depends on $i$, with no additional cost.
        \end{itemize}
    \item Each fact $f$ such that $f[B]=v_1$ is in conflict with the fact $R(v_1,v_1,\val{0})$. This case is symmetric to the previous one, thus we will not elaborate on all of the possible cases.
    \setcounter{counter}{\value{enumi}}
\end{enumerate}
At this point, $J'$ contains facts of the form $R(v_1,v_1,\val{0})$ and $R(v_2,v_2,\val{0})$, facts from $J$ that are not in conflict with these facts, and facts of the form $R(y_i,v_i,\val{0})$. Note that we insert a fact $R(y_i,v_i,\val{0})$ to $J'$ only if there is a fact $R(v_2,v_i,x)$ in $J$ for some $v_i\neq v_2$. Since the fact $R(v_2,v_i,x)$ belongs to $J$, no other fact $f'$ such that $f'[B]=v_i$ also belongs to $J$, unless the facts are identical, and all of these identical facts are replaced by the same fact. Thus, there is no fact $f''$ in $J$, that is not in conflict with one of $R(v_1,v_1,\val{0})$ or $R(v_2,v_2,\val{0})$, such that $f''[B]=v_i$, and the fact $R(y_i,v_i,\val{0})$ agrees on the value of attribute $B$ only with other facts that look exactly the same. Moreover, the fact $R(y_i,v_i,\val{0})$ agrees on the value of attribute $A$ only with other facts that look exactly the same, since we use a new value $y_i$ that does not appear in any other fact in the instance. Thus, no fact $R(y_i,v_i,\val{0})$ is in conflict with the rest of the facts in $J'$, and $J'$ is consistent. Moreover, since we only replaced facts with no additional cost, so far we did not exceed the cost of $J$.

Finally, there are just two more cases that we have not covered yet. Assume that $f$ is the fact $R(v_2,v_i,x)$ for some $v_i\neq v_2$, and assume that the original fact $f$ was the fact $R(v_2,v_i,\val{0})$ and $v_i\neq v_1$ (if $v_i=v_1$ then we have already covered this case). Then, it may be the case that the fact was not updated by $J$ at all. Since the fact $R(v_2,v_i,x)$ belongs to $J$ and $J$ is consistent, no other fact $f'\in J$ is such that $f'[A]=v_2$ (unless they are identical). Thus, $J$ updated the value of attribute $A$ in both $f_3$ (the fact $R(v_2,v_2,\val{1})$) and $f_4$ (the fact $R(v_2,v_1,\val{0})$). As mentioned in the observation at the beginning of this proof, if $J$ updated both these values, then the cost of updating the facts $f_2$, $f_3$ and $f_4$ is at least $5$ (and not at least $4$ as we assumed so far). Thus, in this case, we can use the additional cost that we have, to change one more cell in the fact $R(v_2,v_i,x)$. 

Similarly, if $J$ contains a fact $f$ of the form $R(v_i,v_1,x)$ for some $v_i\neq v_1$, and the original fact $f$ was the fact $R(v_i,v_1,\val{0})$ and $v_i\neq v_2$, then $J$ updated the value of attribute $B$ in in both $f_2$ (the fact $R(v_1,v_1,\val{1})$) and $f_4$ (the fact $R(v_2,v_1,\val{0})$). This again gives us an additional cost to update one more cell in the fact $R(v_i,v_1,x)$. Thus, we will do the following:
\begin{enumerate}
    \setcounter{enumi}{\value{counter}}
    \item If the fact $R(v_2,v_i,x)$ for some $v_i\not\in\set{v_1,v_2}$ belongs to $J$, and the original fact was $R(v_2,v_i,\val{0})$, then we replace this fact in $J'$ with the fact $R(v_2,v_2,\val{0})$ with an additional cost of at most one.
    \item If the fact $R(v_j,v_1,x)$ for some $v_j\not\in\set{v_1,v_2}$ belongs to $J$, and the original fact was $R(v_j,v_1,\val{0})$, then we replace this fact in $J'$ with the fact $R(v_1,v_1,\val{0})$ with an additional cost of at most one.
    \setcounter{counter}{\value{enumi}}
\end{enumerate}
At this point, we have inserted to $J'$ one fact for each fact in $J$, and as explained above, $J'$ is now consistent. Moreover, we never exceeded to the of $J$, thus we found a new v-repair $J'$ that updates each fact updated by $J$, as well as the fact $R(v_1,v_2,\val{0})$ and that concludes our proof of the lemma.
\end{proof}

Lemme~\ref{lemma:comp-proof} implies that for each v-repair $J$ of $I$ that updates $t$ facts of the form $R(v_i,v_j,\val{0})$ for some $t<2|E|$, there is a v-repair $J'$ of $I$, that updates all of the facts of the form $R(v_i,v_j,\val{0})$, such that the cost of $J'$ is lower or equal to the cost of $J$. Thus, each v-repair of $I$ is of cost at least $2|E|$.

Finally, we can prove that no v-repair of $I$ is of cost $2|E|+k$ for some $k<|C_{min}|$. The proof of this part of the lemma is very similar to the proof of~\cite{DBLP:conf/icdt/KolahiL09}. Each v-repair of $I$ has a cost $2|E|+k$ for some $k$. Let us assume, by way of contradiction, that there is a v-repair of $I$ that updates $2|E|+k$ cells, for some $k<|C_{min}|$ (where $C_{min}$ is a minimum vertex cover of $g$). Let $J$ be the minimum v-repair of $I$ (clearly, in this case, $J$ updates $x=2|E|+k'$ cells, for some $k'<|C_{min}|$). Lemma~\ref{lemma:comp-proof} implies that we can assume that $J$ updates all of the facts of the form $R(v_i,v_j,\val{0})$.
Let $\set{f_1,\dots,f_l}$ be the set of facts of the form $R(v_i,v_i,\val{1})$ that are updated by $J$, and let $C'=\set{v_{i_1},\dots,v_{i_l}}$ be the set of the vertices that appear in those facts. Since $J$ updates all of the $2|E|$ facts of the form $R(v_i,v_j,\val{0})$, the cost of $J$ is greater or equal to $2|E|+|C'|$, thus we get that $2|E|+|C_{min}|>2|E|+k'>=2|E|+|C'|$, and $|C'|<|C_{min}|$. Therefore, $C'$ cannot be a cover of $g$ (since the size of the minimum vertex cover is $|C_{min}|$. Thus, there are at least $|C_{min}|-|C'|$ edges $(v_i,v_j)$ in $g$, such that neither $v_i\in C'$ nor $v_j\in C'$ (that is, $J$ doesn't update the fact $R(v_i,v_i,\val{1})$ and also doesn't update the fact $R(v_j,v_j,\val{1})$). For each one of these $|C_{min}|-|C'|$ edges, we have to change at least $4$ cells in the facts $R(v_i,v_j,\val{0})$ and $R(v_j,v_i,\val{0})$ (the values of attributes $A$ and $B$), thus the cost of $J$ is greater or equal to $4(|C_{min}|-|C'|)+2(|E|-(|C_{min}|-|C'|))+|C'|=2|C_{min}|+2|E|-|C'|$. Finally, we get that $2|E|+|C_{min}|>=2|C_{min}|+2|E|-|C'|$, that is $|C'|>=|C_{min}|$, which is a contradiction to the fact that $|C'|<|C_{min}|$.

\subsection{Proof of NP-hardness from Proposition~\ref{prop:quadratic-ratio-U-approx}}

\begin{proposition}\label{prop:NP-hard-quadratic}
Finding an optimal U-repair for $\depset = \set{A_1A_2 \cdots A_k \rightarrow B, B \rightarrow C}$ is NP-hard for all $k \geq 2$.
\end{proposition}

\begin{proof}
We reduce it from the problem of finding an optimal U-repair for $\set{A \rightarrow B, B \rightarrow C}$ on a database $R(A, B, C)$ that has shown to be NP-hard by Kolahi and Laksmanan \cite{DBLP:conf/icdt/KolahiL09}.\\

Given $R(A, B, C)$, we construct $S(A_1, A_2, \cdots, A_k, B, C)$, where for  every tuple $r(a, b, c)$ in $R$, we create a tuple $s(a, 0, 0, \cdots 0, , b, c)$ in $S$, i.e., $A_1 = A$, $B = B, C = C$, and the remaining columns $A_2, \cdots, A_k$ take 0 values in $S$. We claim that $R$ has a consistent update of cost $\leq M$  if and only if $S$ has a consistent update of cost $\leq M$.\\

\textbf{(If):} Suppose $R$ has a consistent update $\hat{R}$ of cost $M$. We can obtain a consistent update $\hat{S}$ of $S$ of the same cost by updating the $A_1, B, C$ values of $S$ as in $R$, and leave $A_2, \cdots, A_k$ unchanged. If $B \rightarrow C$ is violated in $\hat{S}$ for two tuples $s_1, s_2$, they will also be violated for the corresponding tuples $r_1, r_2$ in $\hat{R}$. If $A_1 \cdots A_k \rightarrow B$ is violated for two tuples $s_1, s_2$ in $\hat{S}$, they must have different values of  $B$ but the same value of $A_1\cdots A_k$, i.e. the same value of $A_1 = A$ in $\hat{R}$, violating the FD $A \rightarrow B$ in $\hat{R}$ and contradicting that it is a consistent update of $R$.\\

\textbf{(Only if):} Suppose we have a consistent update $\hat{S}$ of $S$ of cost $M$. \\

(1) First we claim that any tuple $s \in \hat{S}$ updates at most one value of $A_1\cdots A_k$. Otherwise, if there is a tuple $s$ where more than one of these $k$ attributes have been updated, we can always update one of them, say $A_1$, to a new value not used in $\hat{S}$ so far, and satisfy the FD  $A_1A_2 \cdots A_k \rightarrow B$ with less cost (one change instead of $\geq 2$ changes for $s$). Note that this change does not affect the FD $B \rightarrow C$. \\

(2) Next we will update $\hat{S}$ without increasing its cost such that only $A_1, B, C$ attributes are updated, and the other attributes are unchanged.\\

Consider any tuple $s \in \hat{S}$ such that (exactly) one of $A_2 \cdots A_k$ attributes has been changed (assuming (1) holds). Without loss of generality, suppose this attribute is $A_2$, which has received a value $a_2$ after being changed from 0. Hence the cost of changing $a_2$ is 1 for $s$. Instead, we update $A_1$ for this tuple assigning to a fresh new value $a_1$ (not used anywhere else), and keep $A_2$ unchanged to 0. Note that although $a_2$ may have been used in other tuples, $A_1 = a_1$ is a fresh new value, and therefore would not interfere with any other tuple. Moreover, assigning a new value to $A_1$ ensures the FD $A_1A_2 \cdots A_k \rightarrow B$. Like (1), this change does not affect the FD $B \rightarrow C$, and $B, C$ attributes are left unchanged in th repair $\hat{S}$. Further, we do not increase the cost.\\

After applying (1) and (2) to all tuples, we have a solution $\hat{S}$ of cost $\leq M$ where only $A_1, B, C$ are updated. Suppose $\hat{R} = \rho_{A_1 \rightarrow A} [\pi_{A_1 BC} \hat{S}]$ (project to $A_1BC$ and rename $A_1$ to $A$). It  can be seen that this solution satisfies the FDs $B \rightarrow C$ since this FD is maintained in $\hat{S}$. It also satisfies the FD $A \rightarrow B$, since otherwise there are two tuples $r_1, r_2 \in \hat{R}$ with the same value of $A$ and different values of $B$. This implies that the corresponding tuples $s_1, s_2$ in $\widehat{S}$ have the same value of $A_1$ and different values of $B$. Since due to (1), (2), both $s_1, s_2$ have the same values of all attributes in $A_2 \cdots A_k$ (all 0), together with $A_1$, they have the same values of $A_1A_2 \cdots A_k$ but different values of $B$, violating FD  $A_1A_2 \cdots A_k \rightarrow B$, and contradicting the fact that $\hat{S}$ is a consistent update of $S$. Hence we get a consistent update$\hat{R}$ of $R$ of at most cost $M$.
\end{proof}
